# Supplementary material for: Trace Inclusion for One-Counter Nets Revisited
Source: arXiv:1404.5157 source file (2015-04-19)
Supplement: Supplementary file 1 [file appendix.tex]

\lemwitnesspreservation*
\input{proofs/lem_witness_preservation}

\lemruleswqo*
\input{proofs/lem_rules_wqo}

\lembounds*
\input{proofs/lem_bounds}

\thmform*
\begin{proof}
\input{proofs/form}
\end{proof}
